# Supplementary material for: High-angular momentum excitations in collinear antiferromagnet FePS$_3$
Source: arXiv:2212.07221 source file (2022-12-14)
Supplement: Supplementary file 1 [file suppl.pdf]

# *Supplementary Information for:*
# High-angular momentum excitations in collinear antiferromagnet $FePS_3$

Jan Wyzula,[1,2] Ivan Mohelský,[1] Diana Václavková,[1] Piotr Kapuscinski,[1] Martin Veis,[3] Clément Faugeras,[1] Marek Potemski,[1,4] Mike E. Zhitomirsky,[5] and Milan Orlita[1,3]

[1] *Laboratoire National des Champs Magnétiques Intenses, EMFL, CNRS UPR3228, Univ. Grenoble Alpes, Univ. Toulouse, Univ. Toulouse 3, INSA-T, Grenoble and Toulouse, F-38042, France*
[2] *Department of Physics, University of Fribourg, Chemin du Musée 3, CH-1700 Fribourg, Switzerland*
[3] *Institute of Physics, Charles University, Ke Karlovu 5, Prague, CZ-121 16, Czech Republic*
[4] *CENTERA Labs, Institute of High Pressure Physics, PAS, PL-01-142 Warsaw, Poland*
[5] *Univ. Grenoble Alpes, CEA, IRIG, PHELIQS, 17 avenue des Martyrs, F-38000 Grenoble, France*
(Dated: November 22, 2022)

## Spin Hamiltonian and AFMR modes

Here we briefy outline basic steps and main results of the spin-wave calculations for the AFMR spectrum of the zig-zag antiferromagnetic state on a honeycomb lattice realized by iron moments in $FePS_3$. The geometry of the exchange couplings and the resulting zig-zag antiferromagnetic structure are schematically shown in Fig. S1. The magnetic unit cell contains two $\uparrow$ and two $\downarrow$ pointing sublattices that are indexed as shown in Fig. S1.

The microscopic spin Hamiltonian of $FePS_3$ includes Heisenberg exchange interactions and the single-ion anisotropy:

$$\hat{\mathcal{H}} = \sum_{\langle ij\rangle} J_{ij}\mathbf{S}_i\cdot\mathbf{S}_j - D\sum_i (S_i^z)^2 + g\mu_B B\sum_i S_i^z \ , \qquad \text{(S1)}$$

where $J_{ij}$ extend up to the third-neighbor shell. Note that due to a different convention used in writing the spin-pair sums, we need to multiply by a factor of $-2$ the exchange constants deduced by Lancon et al. [1].

The AFMR modes correspond to $k = 0$ excitations. Therefore, instead of studying the full lattice Hamiltonian (S1), we can project it to the four sublattice state:

$$\begin{aligned}\hat{\mathcal{H}} &= J_1\big[2\mathbf{S}_1\cdot\mathbf{S}_2 + 2\mathbf{S}_3\cdot\mathbf{S}_4 + \mathbf{S}_1\cdot\mathbf{S}_3 + \mathbf{S}_2\cdot\mathbf{S}_4\big] + 4J_2\big(\mathbf{S}_1\cdot\mathbf{S}_4 + \mathbf{S}_2\cdot\mathbf{S}_3\big)\\ &+ 3J_3\big(\mathbf{S}_1\cdot\mathbf{S}_3 + \mathbf{S}_2\cdot\mathbf{S}_4\big) - D\big(S_{1z}^2 + S_{2z}^2 + S_{3z}^2 + S_{4z}^2\big) + g\mu_B B\big(S_{1z} + S_{2z} + S_{3z} + S_{4z}\big). \qquad \text{(S2)}\end{aligned}$$

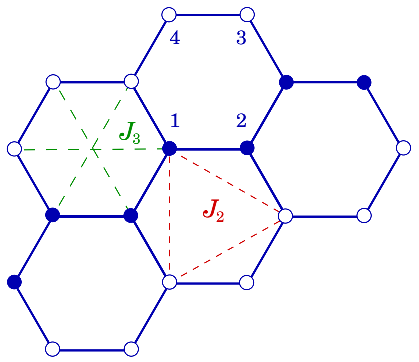


FIG. S1: $J_1$–$J_2$–$J_3$ Heisenberg spin model on a honeycomb lattice. Full and empty circles represent up and down spins in the zig-zag antiferromagnetic structure of $FePS_3$.

We now apply the Holstein-Primakoff transormation for the spin operators and obtain in a quadratic order:

$$\begin{aligned}\hat{\mathcal{H}}_2 &= S(2D + 3J_3 - J_1 + 4J_2)(a_1^\dagger a_1 + a_2^\dagger a_2 + a_3^\dagger a_3 + a_4^\dagger a_4) + g\mu_B B(a_1^\dagger a_1 + a_2^\dagger a_2 - a_3^\dagger a_3 - a_4^\dagger a_4) +\\ &+ 2J_1 S(a_1^\dagger a_2 + a_2^\dagger a_1 + a_3^\dagger a_4 + a_4^\dagger a_2) - (3J_3 + J_1)(a_1 a_3 + a_2 a_4 + a_3^\dagger a_1^\dagger + a_4^\dagger a_2^\dagger)\\ &- 4J_2 S(a_1 a_4 + a_2 a_3 + a_4^\dagger a_1^\dagger + a_3^\dagger a_2^\dagger)\,. \qquad \text{(S3)}\end{aligned}$$

Performing standard steps of diagonalization of such Hamiltonians: (i) introducing symmetric/asymmetric bosons for (1,2) and (3,4) spin pairs and (ii) canonical Bogolyubov transformation we obtain two pairs of AFMR modes. The low-energy symmetric excitations have energy gaps:

$$\Delta_S = 2S\sqrt{D(D+J_1+3J_3+4J_2)} \pm g\mu_B B\,, \tag{S4}$$

whereas the higher-lying antisymmetric modes are given as:

$$\Delta_A = 2S\sqrt{(D-2J_1+4J_2)(D+3J_3-J_1)} \pm g\mu_B B\,. \tag{S5}$$

The $\pm$ signs in the above expression signify that both lower and upper pairs of excitations consist of magnons with $S_z = \pm 1$.

Let us now compute the energy of a fully reversed spin neglecting, at the same time, its dispersion. The energy costs of such an excitation is obtained by counting broken bonds:

$$\Delta_4 = S^2(-2J_1+6J_3+4J_2) \pm 4g\mu_B B\,, \tag{S6}$$

from which we obtain the expression given in the main text.

## Additional observed AFMR-like modes

Besides the resonance modes $M_S$, $M_A$ and $M_4$ discussed in detail in the main text, we have also identified additional AFMR-like spectral features in our data. These include the $M_\alpha$ and $M_\beta$ modes observed nearby the $M_4$ mode and another AFMR-like excitation at lower photon energies denoted as $M_2$. These three additional modes are clearly visible in Fig. S2. Notably, their integral intensities are significantly weaker – approximately by a factor of $10^{-3}$ for the $M_2$ excitation and by a factor of $10^{-4}$ for the $M_\alpha$ and $M_\beta$ modes – as compared to the 1-magnon gaps $M_S$ and $M_A$. The effective $g$ factors extracted from slopes, $g_2 = (4.2 \pm 0.2)$, $g_\alpha = (7.3 \pm 0.5)$ and $g_\beta = (5.0 \pm 0.5)$, provide us with a clear indication of their multi-magnon/multipolar nature. We attribute their appearance in $FePS_3$ to the balance between strong easy-axis anisotropy $D$ and nearest-neighbour ferromagnetic exchange interaction $J_1$.

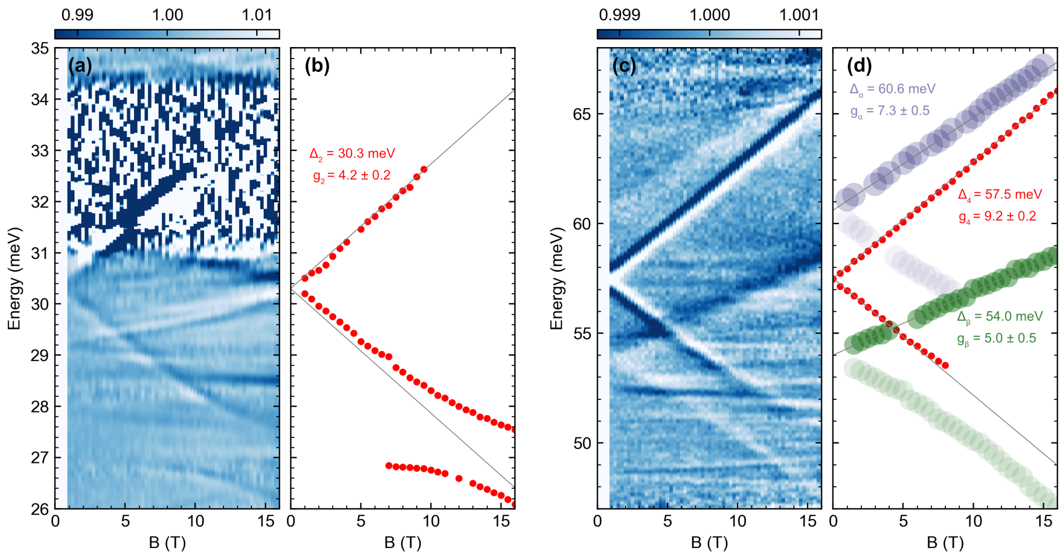


FIG. S2: False-color maps of differential magneto-transmission measured on $FePS_3$ ($T_B/T_{B-\Delta B}$ for $\Delta B = 1$ T, with a step 0.25 T) in two spectral windows in panels (a) and (c). The extracted positions of resonances at selected values of $B$ are plotted in panels (b) and (d), respectively. The size and transparency of the full circles in (d) are chosen to approximately match the error bar and the strength of transitions. The position of resonance at $B = 0$ and the effective $g$ factor were obtained via a fit, using the standard AFRM formula: $\omega_{\mathrm{AFMR}} = \Delta \pm g\mu_B B$. For the weaker $M_\alpha$ and $M_\beta$ resonances, only the upper, significantly more pronounced branch was fitted. One may also observe that the lower branch of the $M_\beta$ mode exhibits slightly non-linear in $B$ evolution.

The $M_2$ mode, characterized by $g_2 = 4.2$ and by the energy of $\Delta_2 = 30.3$ meV, see Fig. S2a,b, corresponds to a quadrupolar excitation of two magnons from the bottom of the 1-magnon band ($\Delta_S = 15.1$ meV). Each magnon in such a pair corresponds to a propagating plane wave. They seem to interact, independently of each other, with an optical phonon mode at 13.5 meV. This gives rise to avoided crossing behavior that is observed for the lower branch of the $M_2$ excitation around the photon energy of 27 meV. Such a coupling is consistent with magnon-phonon interaction observed recently for the lower 1-magnon gap in $FePS_3$ [2, 3]. The pair of magnons can reduce their energy by enhancing a probability for states with two spin flips occupying nearby lattice sites. The binding energy then may shift the 2-magnon excitation below the 2-magnon continuum at $2\Delta_S$. Nevertheless, in this particular case, we find $\Delta_2 \approx 2\Delta_S$ and the binding energy thus seems to be negligible.

The $M_\alpha$ mode, with $g_\alpha = 7.3$ and $\Delta_\alpha = 60.6$ meV, may correspond to a bound complex of three 1-magnon excitations, thus having the octupolar symmetry. The AFMR-like mode $M_\beta$ at $\Delta_\beta = 54.0$ meV exhibits a bit lower effective $g$ factor, $g_\beta = 5.0$, as compared to the $M_\alpha$ mode which may point towards its 2-magnon character. Since the energy $\Delta_\beta$ exceeds the onset of the 2-magnon continuum for the lower 1-magnon gap (*i.e.*, twice $\Delta_S$), it is plausible to assume that the $M_\beta$ mode is a bound state of two magnons from the upper 1-magnon gap. Note that all these modes can further hybridize with conventional 1-magnons and 4-magnon single-ion bound states due to spin-orbit coupling. Widely varying absorption intensities of different resonance modes are determined by matrix elements, which couple the ground state with a given multipolar excitation. Abundance of distinct resonance modes in $FePS_3$ – presented here, but likely also yet to be discovered – makes it an interesting model system for studying nontrivial quantum excitations in almost semiclassical ($S = 2$) magnetic materials.

Let us add that, following the lower branch of the $M_4$ excitation as a function of $B$, we may see that its visibility in the spectra, see Fig. S2c, decreases when it enters the spectral range of 51-54 meV. In this range, we observe weakly $B$-dependent, *i.e.*, nearly horizontal in Fig. S2h, spectral features. We interpret them as multi-phonon resonances which become $B$-dependent due to magnon-phonon coupling (clearly present in $FePS_3$ and studied experimentally see Refs. [2, 3]) and which may effectively broaden/mask the lower branch of the 4-magnon excitation.

---


[1] D. Lancon, H. C. Walker, E. Ressouche, B. Ouladdiaf, K. C. Rule, G. J. McIntyre, T. J. Hicks, H. M. Ronnow, and A. R. Wildes, Phys. Rev. B **94**, 214407 (2016).

[2] Sheng Liu, Andras Granados del Aguila, Dhiman Bhowmick, Chee Kwan Gan, T. Thu Ha Do, M. A. Prosnikov, David Sedmidubsky, Zdenek Sofer, Peter C. M. Christianen, Pinaki Sengupta, and Qihua Xiong, Phys. Rev. Lett. **127**, 097401 (2021).

[3] D. Vaclavkova, M. Palit, J. Wyzula, S. Ghosh, A. Delhomme, S. Maity, P. Kapuscinski, A. Ghosh, M. Veis, M. Grzeszczyk, C. Faugeras, M. Orlita, S. Datta, and M. Potemski, Phys. Rev. B **104**, 134437 (2021).
